# Supplementary material for: Declarative Probabilistic Logic Programming in Discrete-Continuous Domains
Source: arXiv:2302.10674 source file (2024-09-08)
Supplement: Supplementary file 1 [file amc.tex]

\section{Weighted Model Counting and Algebraic Model Counting} \label{app:amc}

Formal logic can be used to describe problems that arise in artificial intelligence. Here we will focus on propositional logic formulas, which we define as follows
\begin{definition}\label{def:preplogic}
	Let $\bvars$ be a set of $M$ Boolean variables.
	We then define propositional logic formulas as Boolean combinations (by means of the standard Boolean operators $\{\neg, \land, \lor, \rightarrow, \leftrightarrow \}$) of {\bf Boolean variables} $b_i \in \bvars$.
\end{definition}

A fundamental question to ask is whether there exists an assignment to the Boolean variables present in the logic formula that satisfies the formula.
% \begin{definition}[Satisfying interpretation of propositional logic formula]
% \label{def:sat_interpretation}
% 	Let ${\bf j}$ and ${\bf k}$ be two disjoint sets of variables and $\phi({\bf j}, {\bf k})$ be a propositional formula over ${\bf j}$ and ${\bf k}$.
% 	The set of total interpretations (or total assignments) that satisfy $\phi$ is the set of assignments to the elements in ${\bf j}$ and ${\bf k}$ that satisfy $\exists {\bf j}, ${\bf k}$:\phi(${\bf j}$,${\bf k}$)$.
% 	We denote the set of total satisfying interpretations (or models) by $\mathcal{I}_{{\bf j},{\bf k}}(\phi)$.
% 	The set of partial interpretations is denoted by $\mathcal{I}_{{\bf j}}(\phi)$, which is the set of assignments to ${\bf j}$ that satisfy $\exists {\bf k}:\phi({\bf j},{\bf k})$.
% 	The set of total assignments to a partially interpreted formula is denoted by $\mathcal{I}_{{\bf j}} (\phi^{\bf k})$, which denotes the set of assignments to the elements in ${\bf j}$ that satisfy $\phi({\bf j},{\bf k}_\inter)$, with ${\bf k}_\inter \in \mathcal{I}_{{\bf k}}(\phi)$. 
% \end{definition}
Determining whether a propositional logic formula is satisfiable is a computational hard problem and falls in the NP-complete complexity class. Nevertheless, a plethora of practical solvers exists (\eg MiniSAT~\citep{sorensson2005minisat}, CryptoSAT~\citep{lafitte2018cryptosat}) that tackle the Boolean satisfiability problem and perform astoundingly well in practice by exploiting structure present in all problems but the most intricate ones. 

We can also ask an other questions: how many distinct assignments satisfy a formula? For propositional logic formulas this simply amounts to counting the number of satisfying assignment to the Boolean variables --  a \#P-complete problem~\citep{valiant1979complexity}. The number of distinct satisfying assignments is dubbed the \textit{model count} and the task of computing the model count is also referred to as $\#SAT$.

Weighted model counting further generalizes \#SAT tasks. Instead of simply counting the number of satisfying assignments, one performs a weighted sum over models.
\begin{definition}[Weighted model counting (WMC)] \label{def:wmc} Given a set $\bvars$ of $M$ Boolean variables, a weight function $w: \mathbb{B}^M \rightarrow \mathbb{R}_{\geq 0}$, and a propositional formula $\support$ over $\bvars$, the {\bf weighted model count} is
	\begin{align}\label{eqn:wmc}
	 \wmc(\support,\weight {\mid} \bvars) = \sum_{\omega \in \mathcal{M}(\phi)} \weight(\omega)
	\end{align}
	$\mathcal{M}(\phi)$ is the set of models of $\support$, \ie the set of interpretations of the Boolean $\bvars$ that satisfy $\support$.
\end{definition}
Traditionally, WMC is used when the weight function $\weight$ factorizes as a product of weights of literals:
\begin{equation}
 \wmc(\support, \weight |\bvars) {=} \sum_{\omega \in \mathcal{M}(\phi)} \prod_{\ell \in \omega} \weight(\ell)
\end{equation}
When performing probabilistic inference, we take
\begin{equation}
0 {\leq} w(b_i){\leq} 1 \quad\text{and}\quad w(b_i){+}w(\neg b_i)=1
\end{equation}
The resulting sum over products is then a computation in the probability semiring~\citep{kimmig2017algebraic}. Effectively, this computes the probability that a propositional logic formula is satisfied.

\citet{kimmig2017algebraic} further generalize probabilistic inference over propositional formulas, \ie over satisfying models, to arbitrary commutative semirings. The general setting of model counting over commutative semirings is called algebraic model counting.
\begin{definition}\label{def:comm_semiring} 
	A {\bf  commutative semiring} is an algebraic structure $(\mathcal{A},\oplus,\otimes,\allowbreak e^{\oplus},e^\otimes)$ equipping a set of elements $\mathcal{A}$ with addition and multiplication such that
	\begin{enumerate}
		\item addition $\oplus$ and multiplication $\otimes$ are binary operations $\mathcal{A}\times \mathcal{A}\rightarrow \mathcal{A}$
		\item addition $\oplus$ and multiplication $\otimes$ are  associative and commutative binary operations over the set $\mathcal{A}$
		\item $\otimes$ distributes over $\oplus$
		\item  $e^\oplus \in \mathcal{A}$ is the neutral element of $\oplus$
		\item  $e^\otimes \in \mathcal{A}$ is the neutral element of $\otimes$
		\item $e^\oplus \in \mathcal{A}$ is an annihilator for $\otimes$
	\end{enumerate}
\end{definition}

\begin{definition}\label{def:amc} (Algebraic model counting (AMC)) \citep{kimmig2017algebraic} Given:
	\begin{itemize}
		\item a propositional logic theory $\phi$ over a set of variables $\bvars$
		\item a commutative semiring $(\mathcal{A},\oplus,\otimes,e^{\oplus},e^\otimes)$
		\item a labeling function $\alpha:\mathcal{L}\rightarrow \mathcal{A}$, mapping literals $\mathcal{L}$ from the variables in $B$ to values from the semiring set $\mathcal{A}$
	\end{itemize} 
	The algebraic model count of a theory $\phi$ is then defined as:
	\begin{align}
	\textstyle \amc(\phi,\alpha | \bvars) = \bigoplus_{b \in \mathcal{I}_\bvars(\phi)} \bigotimes_{b_i \in b} \alpha (b_i)&  \nonumber
	\end{align}
\end{definition}
We use $\alpha$ instead of $w$ and the term label rather than weight to reflect that the elements of the semiring cannot always be interpreted as weights.

Algebraic model counting constitutes a general framework for many common inference tasks in artificial intelligence. Defining an appropriate semiring and labeling functions allows one, for instance, to perform sensitivity analysis, compute gradients or determine the provenance of queries in databases~\citep{kimmig2017algebraic}.
