# Supplementary material for: Declarative Probabilistic Logic Programming in Discrete-Continuous Domains
Source: arXiv:2302.10674 source file (2024-09-08)
Supplement: Supplementary file 2 [file compilation.tex]

\section{Knowledge Compilation and Algebraic Model Counting} \label{app:compilation}

As mentioned in the previous section, model counting is a computationally hard problem, \#P-hard to be precise. Nevertheless practically useful model counters exist. State-of-the-art techniques for solving model counting problems, are based on exhaustive DPLL algorithms~\citep{birnbaum1999good}, which count the number of satisfying assignments to a formula. These solvers can be divided into two classes: the ones that build up a trace of the DPLL search, and the ones that do not. The latter return immediately the model count. The former builds up a diagrammatic representation of the propositional formula over which the model count can be obtained efficiently. By keeping a trace, such \#SAT solvers~\citep{huang2005dpll,oztok2018exhaustive} constitute, in fact, top-down {\em knowledge compilation} schemes.

Knowledge compilation~\citep{darwiche2002knowledge} has emerged as the go-to technique for dealing with the computational intractability of propositional reasoning (\#P-hard~\citep{valiant1979complexity}). The key idea is to split up inference on logical formulas into an \textit{off-line} and an \textit{on-line} step. In the off-line step, a propositional formula is compiled from its source representation into a target representation, in which repeated on-line poly-time inference is available.

\#SAT can also be performed by compiling formulas bottom-up~\citep{choi2013dynamic}. However, it has been shown ~\citep{huang2005dpll,oztok2018exhaustive} that top-down compilation, \ie knowledge compilation through exhaustive DPLL search, outperforms bottom-up compilers.

Similar to model counting, weighted model counting has as well been performed via knowledge compilation, for instance for probabilistic inference in Bayesian networks~\citep{chavira2008probabilistic} or probabilistic programming~\citep{fierens2015inference}.

A popular and well-known target language for the knowledge compilation of propositional formulas are {\em deterministic decomposable negation normal
form} (d-DNNF) formulas~\citep{darwiche2001tractable}
and variations thereof~\citep{bryant1986graph,darwiche2011sdd}.
Boolean formulas in {\em negation normal form}~\citep{darwiche1999compiling} are nested conjunctions and disjunctions that allow negations only to be applied directly to the atoms in the formula.
Determinism and decomposability are two additional properties that we need to impose in order to guarantee tractable probabilistic inference using algebraic model counting.

\begin{definition}[Determinism] An NNF formula is deterministic if and only if for every disjuntion the disjuncts are pairwise logical inconsistent.
\end{definition}

\begin{definition}[Decomposability] An NNF formula is decomposable if and only if for every conjunction the conjuncts do not share any variables.
\end{definition}

\begin{definition}[Smoothness] 
An NNF is smooth if and only if for each disjunction the disjuncts mention the same variables.
\end{definition}

\begin{algorithm}[t]
    \SetKwFunction{EvalFn}{Eval}
    \SetKwProg{Fn}{function}{}{}
    \SetKwProg{ElseComment}{function}{}{}

	\caption{Evaluating a d-DNNF circuit $\Gamma$ for a
		commutative semiring $\mathcal{S}$ and labeling function $\alpha$~\citep{kimmig2017algebraic}.}
	\label{alg:eval}
\Fn{\EvalFn{$\Gamma$,$\mathcal{S}$,$\alpha$}}{
		\If{  $\Gamma$ is a literal node $l$}{ \Return $\alpha(l)$}
		\ElseIf{$\Gamma$ is a disjunction $\bigvee_{i=1}^m \Gamma_i$}
		{\Return $\bigoplus_{i=1}^m$ \EvalFn{($\Gamma_i$,$\mathcal{S}$,$\alpha$}}
		\Else( \tcp*[f]{$\Gamma$ is a conjunction $\bigwedge_{i=1}^m \Gamma_i$}){
		 \Return $\bigotimes_{i=1}^m$ \EvalFn{($\Gamma_i$,$\mathcal{S}$,$\alpha$}}
	}
\end{algorithm}

% 		{$N$ is a conjunction $\bigwedge_{i=1}^mN_i$}

We will also need the notions of {\em sum-neutrality} and {\em consistency preserving}.

%In order to compute algebraic/weighted model counts on a d-DNNF, we additionally need the neutral-sum property.	
\begin{definition}[Neutral-sum property~\citep{kimmig2017algebraic}]\label{lem:nsp} A semiring addition and labeling function pair $(\oplus,\alpha)$ is neutral \emph{if and only if} $\forall b \in \bvars:  \alpha(b)\oplus \alpha(\neg b)=e^\otimes$.
\end{definition}

\begin{definition}[Consistency-preserving property~\citep{kimmig2017algebraic}]\label{lem:con_prev} A semiring multiplication and labeling function pair $(\otimes,\alpha)$ is consistency-preserving \emph{if and only if} $\forall b \in \bvars:  \alpha(b)\otimes \alpha(\neg b)=e^\oplus$.
\end{definition}

\begin{theorem}[AMC on d-DNNF~\citep{kimmig2017algebraic}]
	\label{theo:amc_ddnnf}
Evaluating an sd-DNNF representation of the propositional theory $\phi$, using Algorithm~\ref{alg:eval}
%, for a semiring and labeling function with neutral tuple $(\oplus, \alpha)$
is a correct computation (cf. \citep[Definition 10]{kimmig2017algebraic}) of the algebraic model count.
\end{theorem}

Under the premise that the $\otimes$ and $\oplus$ operations in Algorithm~\ref{alg:eval} can be perform in constant time and that intermediate results are cached, the computation of an algebraic model count on an sd-DNNF is performed in poly-time~\citep{darwiche2002knowledge}.
