# Supplementary material for: Declarative Probabilistic Logic Programming in Discrete-Continuous Domains
Source: arXiv:2302.10674 source file (2024-09-08)
Supplement: Supplementary file 3 [file labeled_propositional_to_SMT.tex]

\section{The Equivalence of Labeled Propositional Formulas and SMT Formulas}
\label{app:labeled_prop_to_SMT}

In Section~\ref{sec:dc2smt} where we describe the conversions performed by the inference algorithm on a queried \dcproblogsty program we used labeled propositional formulas as an intermediate representation. This, however, ignored the arithmetic meaning inherent to the comparison predicates. We will now refine this our understanding of labeled propositional logic formulas by making the link with weighted model integration~\citep{belle2015probabilistic}.

On the logic formula level we have been treating comparisons, \eg, \probloginline{(temp<25.0)}, as purely logical, with no inherent meaning. For instance, we never exploited facts like $(\text{\probloginline{temp<25}} \land \text{\probloginline{temp>30}}) \leftrightarrow \bot $. Only through the labeling function (cf. Definition~\ref{def:labeling_function}) have comparisons been assigned an arithmetic meaning. For instance, the labeling function {\em interprets} the predicate \probloginline{</2} as an arithmetic comparison and the two arguments (\probloginline{temp}, \probloginline{25.0}) as arithmetic expressions.\footnote{Note that logic programming languages, such as \problogsty, often include a non-logical external arithmetics engine. Through such engines logic programming languages are capable of interpreting arithmetic expressions and comparison predicates, \eg \probloginline{25>5+2} and assign a logical meaning to the comparison~\citep[Section 8]{sterling1994art}. In a sense, probabilistic logic programming languages extend logic programming with probabilistic arithmetics engines.}

Interpreting comparisons can also be performed on the formula level, without the use of labeled atoms. Such formulas are called satisfiability modulo theory (SMT) formulas and extend propositional logic with interpreted first-order predicates. 
% We give a formal definition of SMT formulas in Appendix~\ref{app:wmi} and refer the reader to~\citet{barrett2009handbook} for an in-depth treatment.
% Using the so-called refinement operation one can obtain SMT formulas from Boolean formulas~\citep{barrett2009handbook}.
We refer the reader to~\citet{barrett2009handbook} for a formal definition and in-depth treatment of SMT formulas.
Using the so-called refinement operation one can obtain SMT formulas from Boolean formulas.

\begin{example}[Refinement of a Boolean Formula]\label{example:refinment}
Consider the Boolean formula $\support_g $ from Example~\ref{example:dc2bool}, \ie,:
	\begin{align}
		%\support_g  \nonumber
		%&\leftrightarrow
		&\Big( \phi_{\text{\probloginline{works(1)}}} \leftrightarrow \phi_{\text{\probloginline{cool(1)}}} 
		\lor \phi_\text{\probloginline{hot}} \land  \phi_\text{\probloginline{temp(hot)<25.0}}  
		\lor\neg \phi_\text{\probloginline{hot}}  \land \phi_\text{\probloginline{temp(not_hot)<25.0}}   \Big)  \nonumber \\
	\land ~~	& \Big(
		  \phi_{\text{\probloginline{cool(1)}}} \leftrightarrow  \phi_{\text{\probloginline{rv_cool(1)=:=1}}} \Big) \nonumber \\
	\land ~~ 	& \Big(
		  \phi_\text{\probloginline{hot}} \leftrightarrow \phi_{\text{\probloginline{rv_hot}=:=1}} \Big)
	\end{align}
Refining the Boolean literals that encode a comparison in \dcproblogsty yields the following SMT formula $\support_g ^\uparrow$:
\begin{align}
	%	\support_g ^\uparrow \nonumber
	%	&\leftrightarrow
		&\Big( \phi_{\text{\probloginline{works(1)}}} \leftrightarrow \phi_{\text{\probloginline{cool(1)}}} 
		\lor \phi_\text{\probloginline{hot}} \land  (temp_{hot}{<}25.0)  
		\lor\neg \phi_\text{\probloginline{hot}}  \land  (temp_{not\_hot}{<}25.0)    \Big) \nonumber \\
	\land ~~ 		& \Big( 
		  \phi_{\text{\probloginline{cool(1)}}} \leftrightarrow (rv\_cool_1=1)\Big) \nonumber \\
		\land ~~ 	& \Big( 
		  \phi_\text{\probloginline{hot}} \leftrightarrow  (rv\_hot=1)\Big)
\end{align}
Here the $\uparrow$ in $\support_g ^\uparrow$ indicates that the formula is the refinement of $\support_g $. The formula $\support_g ^{\uparrow}$ is now an SMT formula over the propositional variables 
$\phi_{\text{\probloginline{works(1)}}}$, $\phi_{\text{\probloginline{cool(1)}}}$  and $\phi_\text{\probloginline{hot}}$, the binary SMT variables $rv\_cool_1$ and $rv\_hot$, and the real-valued SMT variables $temp_{hot}$ and $temp_{not\_hot}$.
\end{example}

\begin{example}[Abstraction of SMT Formula]\label{ex:abstraction}
The process of going from an SMT formula back to a propositional logic formula is called abstraction and we denote it by $\downarrow$. If we have, for instance, the SMT formula $\phi$ defined as 
\begin{align*}
    \phi_{\text{\probloginline{cool(1)}}} \lor \phi_\text{\probloginline{hot}} \land  (temp_{hot}{<}25.0)
\end{align*}
we obtain the corresponding propositional formula $\phi^\downarrow$ as:
\begin{align*}
		 \phi_{\text{\probloginline{cool(1)}}} 
		\lor \phi_\text{\probloginline{hot}} \land  \phi_\text{\probloginline{temp(hot)<25.0}}  
\end{align*}
\end{example}

An obvious query to pose is that of the satisfiability of an SMT formula, \ie to figure out whether there is a satisfying assignment to the variables in an SMT formula (\eg~\citep{demoura2009z3}). An equally important query, however, is the weighted counting problem on SMT formulas, which was dubbed {\em weighted model integration}~\citep{belle2015probabilistic}.
% We include a primer on weighted model integration in Appendix~\ref{app:wmi} and refer the reader to the survey paper of~\citet{morettin2021hybrid} for an overview of the field.
We refer the reader to the survey paper of~\citet{morettin2021hybrid} for an overview of the field.
% Recently, \citet{miosic2021measure} also gave a stringent measure theoretic formulation of weighted model integration. 

Under the assumption that the values of the variables in an SMT formula are distributed according to a given probability distribution, the weighted model integral of an SMT formula is identical to the expected value of the SMT formula with  respect to the probability distributions of its variables.
This observation gives us the following Lemma~\ref{lemma:expt_label2wmi}.

\begin{lemma}[The Expected Label as a WMI Problem] \label{lemma:expt_label2wmi}
Let $\phi$ denote the logic propositional formula derived from a relevant ground program $\dcpprogram_g$ with evidence asserted, and let $\alpha$ be the labeling function as defined in Definition~\ref{def:labeling_function}. Computing the expected value of the label of $\phi$ is a weighted model integration problem.
\end{lemma}
\begin{proof}[Proof.] We start by expressing the expected value of the label of a specific $\omega$ in terms of Iverson brackets (Equation~\ref{proof:label_wmieq:iverson}). We then rewrite the integral by putting the Iverson brackets in the boundary of the integral (Equation~\ref{proof:label_wmieq:boundary1}) and slightly rewrite the boundary (Equation~\ref{proof:label_wmieq:boundary2}).
\begin{align}
    &\E_{vars(\omega) \sim  \dcpprogram_g} [\alpha( \omega )] \nonumber \\
    &=
    \int
        \left( \prod_{i: a_i \in CA^+(\omega)} \ive{  c_i(vars(a_i)) } \right)
        \left( \prod_{i: a_i \in CA^-(\omega)} \ive{  \neg c_i(vars(a_i)) } \right) 
    dP_{vars(\omega)}(\omega) \label{proof:label_wmieq:iverson} \\
    &= \int_{\{ a_i^\uparrow: a_i \in CA^+(\omega) \} \cup \{a_i^\uparrow : a_j \in CA^-(\omega)\} }     dP_{vars(\omega)}(\omega)   \label{proof:label_wmieq:boundary1} \\
    &= \int_{ \{  a_i^\uparrow : a_i \in ( CA^+(\omega) \cup CA^-(\omega) )   \} } dP_{vars(\omega)}(\omega)  \label{proof:label_wmieq:boundary2}
\end{align}

To get the expected value of the label of $\phi$ we sum over all $\omega \in ENUM(\phi)$ (Equation~\ref{proof:label_wmieq:expected_label_formula}). We then rewrite the expected label in terms of the Lebesgue measure $\lambda$ and a counting measure $\xi$ for integer variables (Equation~\ref{proof:label_wmieq:product_measure}). We refer to~\citep[Section 4.2]{,miosic2021measure} for a stringent measure theoretic formulation of weighted model integration. Note how we now explicitly integrate over the function $w_\omega$ representing the probability distributions and which was hidden before in the measure $P_{vars(\omega)}$. Referring again to~\citep{miosic2021measure}, we equate Equation~\ref{proof:label_wmieq:product_measure} with the measure theoretic formulation of weighted model integration (Equation~\ref{proof:label_wmieq:wmi}).
\begin{align}
    &\sum_{\omega \in ENUM(\phi) } \int_{ \{  a_i^\uparrow : a_i \in ( CA^+(\omega) \cup CA^-(\omega) )   \} } dP_{vars(\omega)}(\omega) \label{proof:label_wmieq:expected_label_formula}   \\
    &= \sum_{\omega \in ENUM(\phi) } \int_{ \{  a_i^\uparrow : a_i \in ( CA^+(\omega) \cup CA^-(\omega) )   \} } \weight_{\omega} d( \lambda \times \xi) \label{proof:label_wmieq:product_measure}\\
    &=\int_{\mathcal{M}(\phi^\uparrow)} w d(\lambda\times \xi \times \mu)\\
    &= \lwmi(\phi^\uparrow,w) \label{proof:label_wmieq:wmi}
\end{align}
In the second but last line the integration goes over all models of the SMT formula $\phi^\uparrow$ using the product measure $\lambda\times \xi \times \mu$, where $\mu$ is a counting measure for the Boolean variables in $\phi^\uparrow$ (cf.~\citep[Definition 8]{,miosic2021measure}). This then corresponds to the definition of the measure theoretic formulation of WMI, denoted in Equation~\ref{proof:label_wmieq:wmi} by $\lwmi$ (the `L' stands for Lebesgue integration).
\end{proof}

Lemma~\ref{lemma:expt_label2wmi} has the delightful property of  allowing us to compute the expected value of the label of a Boolean formula by adopting inference algorithms that have been developed as approaches to weighted model integration~\citep{sanner2011symbolic,morettin2017efficient,kolb2018efficient,zuidbergdosmartires2019exact,kolb2019exploit,zeng2019efficient,derkinderen2020ordering,zeng2020probabilistic}.

% This means that we can reduce inference in \dcproblogsty to weighted model integration. 
